# Supplementary material for: AnyTaskTune: Advanced Domain-Specific Solutions through Task-Fine-Tuning
Source: arXiv:2407.07094 source file (2024-07-09)
Supplement: Supplementary file 1 [file 800_appendix.tex]

\section{Attribute Prediction Loss} \label{app:attr}

For each augmented DataGraph $\gG^\mathit{aug}$, the certain node features $F_v$ are masked during MaskNode augmentation.
Therefore, we can reconstruct them using the learned embedding $E_v$ with a MLP and train with MSE reconstruction Loss.
$$\gL_{attr}(\gG^\mathit{aug}) = \frac{1}{|\dV|}\sum_v \texttt{MSE}(F_v, \texttt{MLP}(E_v))$$

\section{Dataset Statistics}
\label{app:ds_stats}
 
\begin{table*}[thb]
    \centering
    \caption{Dataset statistics}
    \label{tab:data_stats}
    \begin{tabular}{l|ccc}
    \toprule
        Dataset & \# Nodes & \# Edges & \# Classes \\
    \midrule
        MAG240M & 122M & 1.3B & 153 \\
        Wiki & 4.8M & 5.9M & 639 \\
        arXiv & 169K & 1.2M & 40 \\
        ConceptNet & 791K & 2.5M & 14\\
        FB15K-237 & 15K & 268K & 200 \\
        NELL & 69K & 181K & 291 \\
    \bottomrule
    \end{tabular}
\end{table*}

\section{Task Graph GNN Architecture} \label{architecture}

For the GNN over task graph $M_\texttt{T}$, we use an attention-based GNN, where each node performs attention to other nodes at each layer:

\begin{align}
\beta_{ij} &= \mathit{MLP}\left( W_q^TH^{l}_i || W_k^TH^{l}_j || e_{ij}\right)\\
\alpha_{ij} &= \frac{\exp(\beta_{ij})}{\sum_{k \in \mathcal{N}(i) \cup \{i\}} \exp(\beta_{ik})} \\
H^{l+1}_i &=  \mathit{ReLU}\left(\mathit{BN}\left(H^{l}_i + W_o^T \sum_{j \in \mathcal{N}(i) \cup \{i\}}  \alpha_{ij} W_v^TH^{l}_j \right)\right)
\end{align}

\section{Hyperparameters}

\subsection{Model Architecture, MAG240M and arxiv}
We initialize the node features in citation network datasets using a pretrained language model (RoBERTa \cite{roberta} base model trained on NLI and STSB).The architecture of our PromptGraph model in all of our proposed methods for citation network datasets (full \methodname, PG-NM, and PG-MT) and the baseline (NoPretrain), consists of two message passing layers, $M_\texttt{D}$, over the DataGraph and one message passing layer, $M_\texttt{T}$, over the TaskGraph. These layers are defined in Section 3.1.

For the Contrastive method, the architecture includes two message passing layers, $M_d$, over the DataGraph, and a contrastive learning component that is defined in Section 4.1. The mode for Finetune is the same as the Contrastive method, with the addition of a linear layer head over the output of the two $M_d$ layers, also described in Section 4.1.

\subsection{Model Architecture, knowledge graph datasets}

We initialize node and edge features in knowledge graph datasets using a pretrained language model (MPNet \cite{mpnet}). The architecture of our PromptGraph model in all of our proposed methods for knowledge graph datasets (full \methodname, PG-NM, and PG-MT) and the baseline (NoPretrain), consists of two message passing layers, $M_\texttt{D}$, over the DataGraph, an aggregator as described by Equation \ref{eqn:pooling_kgs}, and two message passing layers, $M_\texttt{T}$, over the TaskGraph, which only pass messages along the positive and query edges. These layers are defined in Section 3.1.

For the Contrastive method, the architecture includes two message passing layers, $M_d$, over the DataGraph, an aggregator as described by Equation \ref{eqn:pooling_kgs} and a contrastive learning component that is defined in Section 4.1. The mode for Finetune is the same as the Contrastive method, with the addition of a linear layer head over the output of the two $M_d$ layers, also described in Section 4.1.

\subsection{Training, MAG240M}

The following describes our pretraining setup:

The pretraining task we used consisted of 30 ways, 3 shots, and 4 queries per task. This specific task configuration was carefully selected to strike a balance between complexity and diversity in the training data, without overwhelming the GPU memory.

We checkpoint the model every 500 steps.

Our pretraining setup included a model with an input dimension of 768 and an embedding dimension of 256, batch size of 1, and the AdamW optimizer with a learning rate of $1 \times 10^{-3}$ and weight decay of $1 \times 10^{-3}$, a pretraining task with 30 ways, 3 shots, and 4 queries per task, and checkpointing every 500 steps. This consistent configuration was applied across all the methods for fair comparison. Our full \methodname setup, on average, involves sampling 1 Neighbor Matching task per 1 multitask pretraining tasks.

For our evaluation process, we computed zero-shot transfer performance of the model on the test set, using the pretraining checkpoint at the 10,000 step of pretraining. The evaluation was conducted on 500 test tasks, with batch size of 5, measured on the downstream task of graph classification accuracy. To maintain consistency, we kept the number of shots and queries constant at 3 for all evaluation tasks.

\subsection{Training, Wiki}

The following describes our pretraining setup:

Our pretraining setup included a model with an input dimension of 768 and an embedding dimension of 256, the AdamW optimizer with a learning rate of $1 \times 10^{-3}$ and weight decay of $1 \times 10^{-3}$, a pretraining task with 30 ways, 3 shots, and 4 queries per task, using a batch size of 10, and checkpointing every 500 steps. This specific task configuration was carefully selected to strike a balance between complexity and diversity in the training data, without overwhelming the GPU memory. This consistent configuration was applied across all the methods for fair comparison. Our full \methodname  setup involves sampling one neighbor matching task per 50 multitask pretraining tasks. 

For our evaluation process, we computed zero-shot transfer performance of the model on the test set, using the pretraining checkpoint at the 8,000 step of pretraining. The evaluation was conducted on 500 test tasks, with batch size of 1, measured on the downstream task of graph classification accuracy. To maintain consistency, we kept the number of shots and queries constant at 3 for all evaluation tasks. We sample 1-hop neighbourhoods for ConceptNet and FB15K-237 and 2-hop neigbourhoods for NELL and Wiki.

% S2,U,A for contrastive
% S2, U, M rest
\section{Ablation on Table \ref{tab:fsnm_ablation} for the PG-NM setting}
\label{app:fsnm_ablation}

\begin{table}[t]
\centering
\caption{Ablation of PG-NM on arXiv.}
\begin{tabular}{l|ccccc c}
\toprule
Ways & PG-NM & 3 $\to$1 shot & No Attr & No Aug & No Attr, Aug & No Attr, Aug, $M_\texttt{T}$ \\
\midrule
3 & \textbf{72.50 $\pm$ \tiny{0.35}}& 69.13 $\pm$ \tiny{1.09} & 65.74 $\pm$ \tiny{1.12} & 68.98 $\pm$ \tiny{1.09} & 66.53 $\pm$ \tiny{1.12} & 63.60 $\pm$ \tiny{1.06} \\
5 & \textbf{61.21 $\pm$ \tiny{0.29}}& 57.49 $\pm$ \tiny{0.92} & 52.78 $\pm$ \tiny{0.90} & 57.50 $\pm$ \tiny{0.85} & 53.89 $\pm$ \tiny{0.92} & 51.27 $\pm$ \tiny{0.69} \\
10 & \textbf{46.12 $\pm$ \tiny{0.19}} &42.03 $\pm$ \tiny{0.60}& 37.99 $\pm$ \tiny{0.63} & 42.43 $\pm$ \tiny{0.64} & 38.87 $\pm$ \tiny{0.59} & 37.62 $\pm$ \tiny{0.34} \\
20 & \textbf{33.71 $\pm$ \tiny{0.11}}& 30.18 $\pm$ \tiny{0.38} & 26.60 $\pm$ \tiny{0.36} & 30.89 $\pm$ \tiny{0.38} & 27.50 $\pm$ \tiny{0.36} & 27.44 $\pm$ \tiny{0.17} \\
40 & \textbf{23.69 $\pm$ \tiny{0.07}} &21.44 $\pm$ \tiny{0.22} & 18.03 $\pm$ \tiny{0.21} & 21.97 $\pm$ \tiny{0.24} & 18.52 $\pm$ \tiny{0.22} & 19.69 $\pm$ \tiny{0.08} \\
\bottomrule
\end{tabular}
\label{tab:fsnm_ablation}
\end{table}

In Table \ref{tab:fsnm_ablation}, we ablate on various configurations of the self-supervised objective PG-NM. As described in Section \ref{sec:objective}, PG-NM is composed of an attribute prediction loss, dropnode and zeronode augmentations, with the default setting of sampling 3 shots neighbor matching tasks. Our best setting, referred to as simply ``PG-NM'', is also shown in Table 1 and comprises of attribute prediction, dropnode and zeronode augmentations, with the default setting of 3 shots.

The ablation results reveal that using all of these elements together results in the highest performance. Specifically, attribute prediction has the greatest impact on PG-NM's performance, as its removal results in an average 7\% drop across all ways, as shown in the `No-Attr' column.

Removing the dropnode and zeronode augmentations results in an average 3\% drop across all ways, as shown in the No Aug' column. Removing both attribute prediction and augmentations results in performance that is similar to just removing attribute prediction alone, which is also roughly a 7\% drop across all ways, as shown in the `No Attr, Aug' column. Additionally, we found that decreasing the number of shots to 1 from the default setting of 3 resulted in an average 3.5\% drop across all ways, as shown.

\section{Evaluation using different numbers of shots} \label{sec:more_shots}

We show evaluation using different numbers of shots, as shown in Figures \ref{fig:cn_more_shots}, \ref{fig:fb_more_shots}, and \ref{fig:nell_more_shots}, \ref{fig:shot}.

\begin{figure}[tbh]
    \centering
    \includegraphics[width=0.6\linewidth]{FB15K-23720_with_errors.pdf}
    \caption{In-context learning accuracy on FB15K-237 in a 20-ways setting  wrt. the number of prompt examples (shots).}
    \label{fig:fb_more_shots}
\end{figure}
\begin{figure}[tbh]
    \centering
    \includegraphics[width=0.6\linewidth]{NELL20_with_errors.pdf}
    \caption{In-context learning accuracy on NELL in a 20-ways setting  wrt. the number of prompt examples (shots).}
    \label{fig:nell_more_shots}
\end{figure}
\begin{figure}[tbh]
    \centering
    \includegraphics[width=0.6\linewidth]{shot.pdf}
    \caption{In-context learning accuracy on arXiv in a 5-ways setting  wrt. the number of prompt examples (shots).}
    \label{fig:shot}
\end{figure}

\section{Scaling with Data Size} \label{sec:scale}

We explore how the model scales with more pretraining tasks.
Note that we use the number of train steps as a proxy because the model sees more pretraining tasks as the training proceeds with almost no redundancy (0.20\% for 10k tasks).
The result on arXiv in a 5-ways setting is illustrated in Figure~\ref{fig:step}.
It shows that the Contrastive baseline saturates quickly and its performance fluctuates given more pretraining tasks.
Instead, \methodname consistently shows an improvement in performance as more data is pretrained on. 

\section{Compute}
We use one NVIDIA A100-SXM4-80GB GPU for all our experiments. One pretrain run of 10k steps takes 3 to 4 hours.

\section{Broader Impacts}
Our work aims to extend the success of in-context learning to graphs and start building toward graph foundation models. This would allow cost-effective and accurate predictions, especially in  domains where labeled data is scarce and long tail such as network anomaly detection,  rare disease diagnosis/treatment, supply chain disruption, and recommendations for new users. However, overreliance on prior knowledge from pretraining could also lead to increased social bias and unfair benefits to the dominate groups. To mitigate this, pretraining data should be diverse and well-balanced, and the pretrained models should be tested on downstream tasks over different groups and subdistributions.
